# Supplementary material for: Issue Link Label Recovery and Prediction for Open Source Software
Source: arXiv:2108.04415 source file (2021-08-10)
Supplement: Supplementary file 1 [file additional_data.tex]

\section{Modelling Additional Data for Link Semantic Recovery}
\label{sec:additionalEncoding}
In the previous section, we explored the use of machine learning techniques for the task of link semantic recovery. We observed that maximal weighted F1 scores were as high as $0.581-0.709$ for three projects when using solely textual issue summaries and descriptions.
%Additionally, we observed that hyper-parameter tuning reduces the variance in classifier performance. 
In this section, we seek to improve recovery performance by incorporating additional data. %Towards this end, we use the technique called of feature representation \cite{cherkauer1994selecting}. The key idea is that to achieve optimal machine learning performance, it is important to choose or construct features that contain all the requisite information to predict the target.
We approach this from two perspectives. Firstly, we consider that the textual features constructed according to the TF-IDF formula may be inadequate for the semantic recovery task. Secondly, the textual content alone might not be sufficient to reliably predict the link semantics. 

We therefore aim to address the final research question (\textbf{RQ3}: to what extent can we recover link semantics using additional information including the textual content external to the issue tracker and the context or metadata contained in issue links?) by incorporating both constructed features relating to textual content external to the issue tracker, and additional measured features using the metadata contained in the issue links.

\subsection{Word Embedding as Text Encoding}
\label{sec:issue_encoding}

% \jg{Still need some work here... for the word embedding}

Firstly, we investigate alternative text encoding functions using word embedding techniques. Word embedding refers to the process of transforming continuous vector representations of words from a high-dimensional space to one with much fewer dimensions \cite{mikolov2013efficient}. This has historically been accomplished using general vector dimensionality reduction techniques such as principal component analysis \cite{jolliffe2011principal} or singular value decomposition for the purposes of latent semantic analysis \cite{landauer1997solution} for the purposes of information retrieval. The word vectors in the embedding space, which are also called word embeddings, can capture several important syntactic and semantic properties of the words when they are trained to build a language model using a large collection of documents. Using word embeddings as input has been shown to greatly improve performance in many natural language processing related tasks such as image captioning \cite{karpathy2015deep} and sentiment analysis \cite{nakov2016semeval}.

When training word embeddings, we primarily take advantage of the fact that there is a large amount of text about general concepts, software development and specific open source projects online. Open source projects in particular have public repositories of textual information describing their processes, components, discussions, and design decisions. Those document collections can be used to pre-train the word embeddings to capture the distribution of word usage in a different context. The word embeddings can then be updated to fit the issue text for each project.

To compare the effectiveness of pre-training word embeddings using different resources for the link semantic recovery task, we consider the following document collections in our study, with varying levels of relevance to the domain:

\begin{enumerate}
    \item Wikipedia: We use the wikitext103 dataset \cite{DBLP:journals/corr/MerityXBS16} which consists of a text dump of generally verified Wikipedia articles that is over 103 million words in size. Despite the fact that this dataset is not directly related to the domain of our projects, we include it because previous work has demonstrated that word embeddings trained on this dataset can effectively capture the statistical distribution of general terms.
    \item Stack Overflow: We use the publicly available StackSample dataset\footnote{https://www.kaggle.com/stackoverflow/stacksample} which contained $10\%$ of Stack Overflow questions and answers as of 2016 %not restricted to a particular language or software domain. 
    We include this dataset because the previous study has suggested that software-specific documents might be more effective than general-purpose corpus to capture word similarities for tasks that rely on processing textual software artifacts \cite{Tian:2014:SSW:2591062.2591071}.
    \item Project Documentation: We additionally use the Cwiki pages of each project in our case study\footnote{https://cwiki.apache.org/confluence/collector/pages.action? \newline key=\{FLEX/Ambari/Hive\}}. These pages contain information such as documentation, release notes, announcements, reference guides, and frequently asked questions. These were mined using the selenium webdriver tool\footnote{https://www.seleniumhq.org/projects/webdriver/}. We aim to explore the potential of capturing project specific context for link semantic recovery through word embedding techniques. We mine a total of $247$ pages from the Ambari project, $327$ from the Flex project and $57$ from the Hive project.
\end{enumerate}

We represent each word in the dataset vocabulary as a fixed-sized dimensional fastText \cite{fastText} embedding. The fastText embedding type was chosen because it additionally accounts for the co-occurrence of sub-word tokens (i.e. groups of characters), and introduces various optimizations for training speed. To aggregate a document's word vectors we average the word embedding vectors, which is a technique known as a Bag of Vectors \cite{P18-1198}.

In summary, the complete issue text encoding process is comprised of two steps: 1. we first use the document collections above to train a set of word embeddings: \textit{\{wiki, stack, proj\}}; 2. then we update the embeddings by training using the same objective on the respective project's issue text (summaries and descriptions). The word embedding text encoding techniques pre-trained by Wikipedia, Stack Overflow, and project documentation are denoted by $textEnc_{wiki}$, $textEnc_{stack}$ and $textEnc_{proj}$ respectively.

\begin{figure}[!b]
    \centering
    \includegraphics[width=0.45\textwidth]{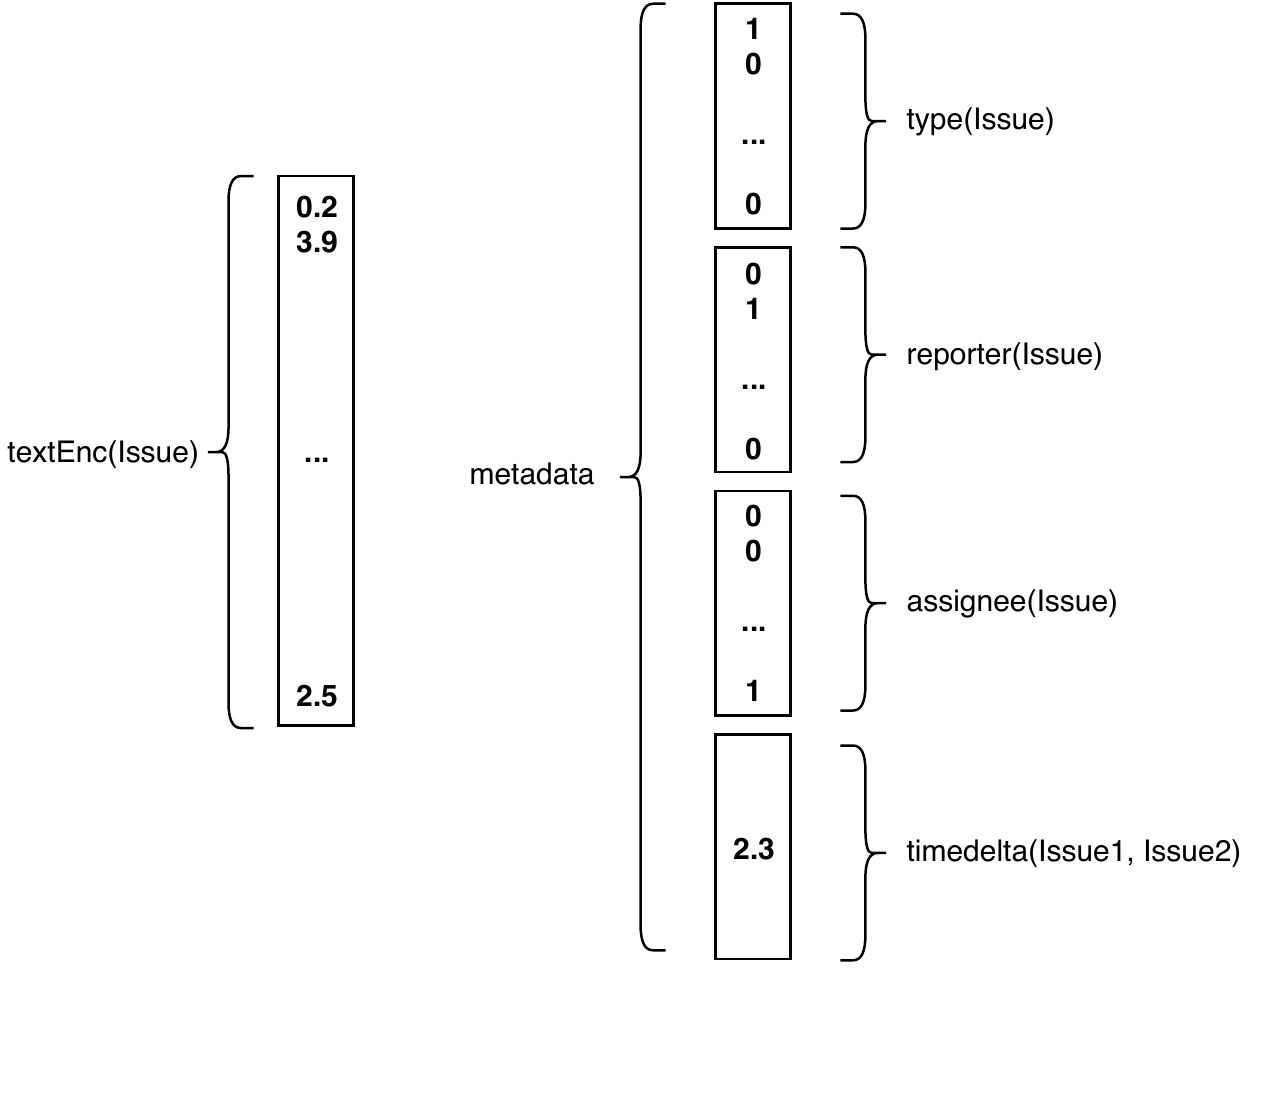}
    \caption{Complete feature-sets for issue link encoding}
    \label{fig:features}
\end{figure}

\subsection{Metadata}
\label{subsec:metadata}

Secondly, we extract additional metadata from the issue tracking system. Our hypothesis is that %the complex interactions that link labels emerge from may co-relate with more than just the text contained in issues. In particular, we include the following metadata items:
the reason for assigning certain link labels may be correlated with the contextual information of the linked issues. This contextual information can be extracted through the issue metadata. In particular, we include the following metadata items:

\begin{enumerate}
    \item $timeDelta(issue_1, issue_2)$: The difference in days between the creation of $issue_1$, and $issue_2$ respectively. These values are scale-normalized by subtracting the mean and dividing by standard deviation;
    \item $type(issue)$: The issue type (see Table \ref{table:typebreakdown});
    \item $assignee(issue)$: The unique identifier of the user to whom this issue is assigned. An additional special identifier is used for no assignee.
    \item $reporter(issue)$: The unique identifier of the user who reported the issue.
\end{enumerate}

This metadata is then transformed into a feature-set. The categorical metadata items such as type, assignee, and reporter are all represented as $N$-dimensional one-hot vectors, where $N$ is the number of categories, that contains $0$ in all indexes except the index corresponding to the category in question which contains $1$.

The complete sets of features (see Figure \ref{fig:features}), including the feature set of the metadata and the text encoding features, are concatenated and then fed into the statistical classifiers introduced in the Section \ref{subsec:mlclassifoverview}.

\subsection{Experiment Setup}
We first use the same text pre-processing steps described in Section \ref{sec:datapreprocess} to prepare three additional text datasets, i.e. Wikipedia, Stack Overflow and Project Documentation. In total we now have four text encoding functions i.e. $textEnc_{wiki}$, $textEnc_{stack}$, $textEnc_{proj}$, and $textEnc_{tfidf}$, which was previously described in Section \ref{subsubsec:tfidf_encoding}. For the embedding-based encoding functions we specify $300$ as the number of dimensions for a single issue vector. 
After the text encoding, we consider the variations of concatenating and not concatenating metadata encoding. 
For each optimization technique discussed in Section \ref{subsec:hpram_search}, the input is a vector resulting from running the encoding function on both issues as well as the optional metadata feature vectors (see Figure \ref{fig:features}). Additionally, we experiment with using only the metadata feature vectors and no textual encoding. We depict the complete process of link semantic recovery in Figure \ref{fig:process_pipeline}.

% We represent each word in the dataset vocabulary as a $300$-dimensional fastText embedding. The fastText embedding type was chosen because it additionally accounts for the co-occurrence of sub-word tokens (i.e. groups of characters), and introduces various optimizations for training speed. To aggregate a document's word vectors we average the word embedding vectors, which is a technique known as a Bag of Vectors \cite{P18-1198}.

\subsection{Experiment Results}

\begin{figure}[!t]
    \centering
    \includegraphics[width=0.49\textwidth]{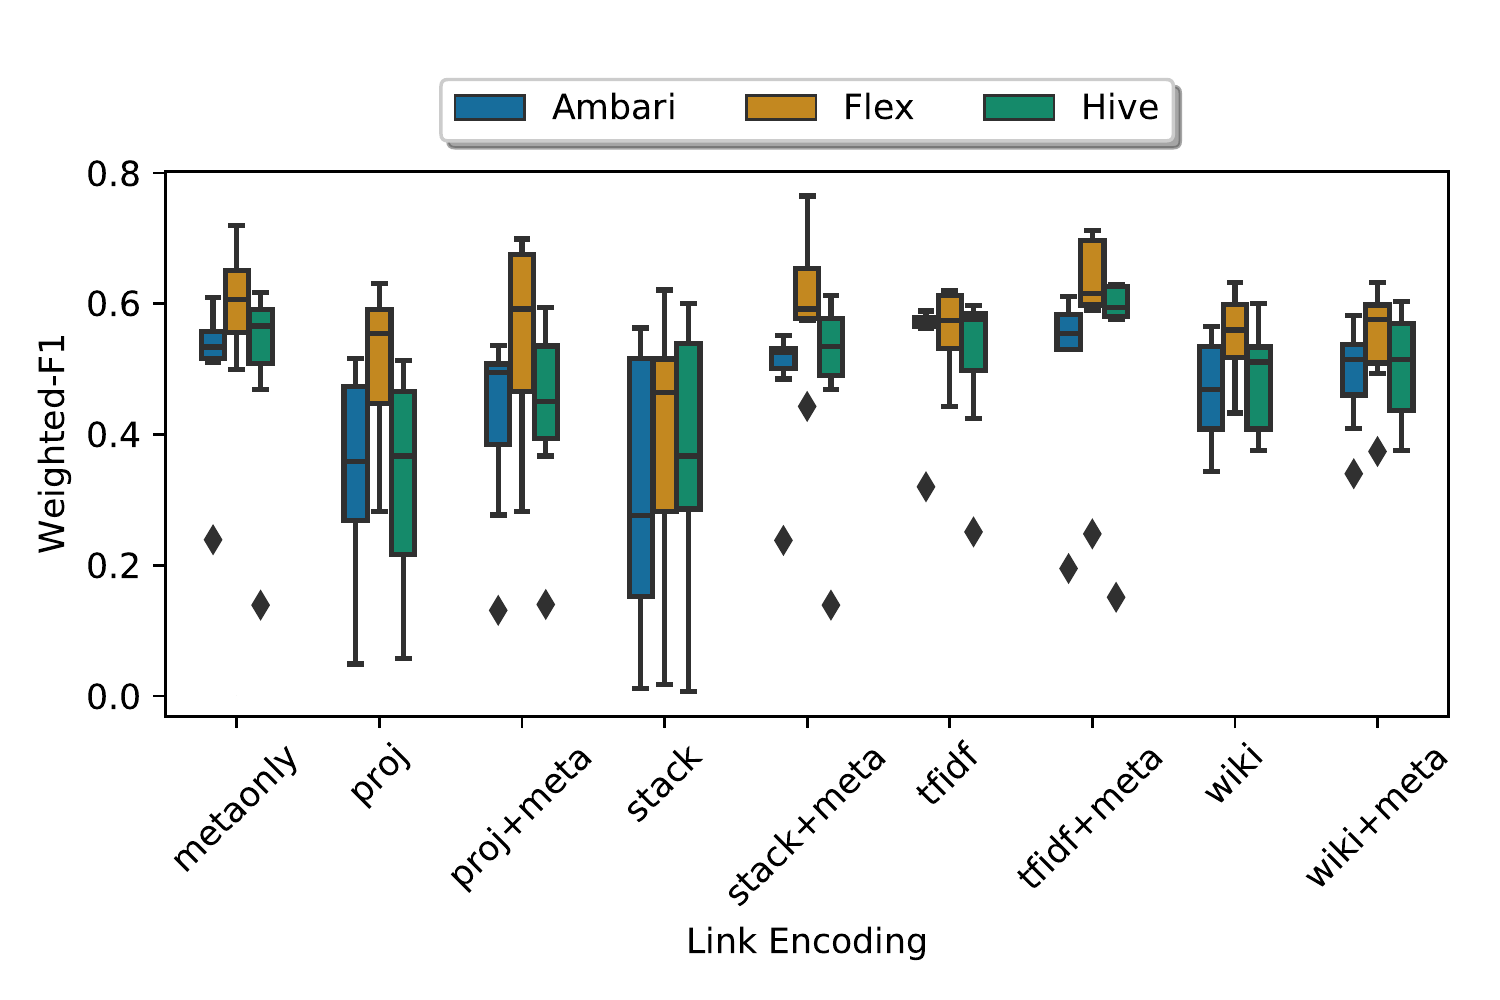}
    \caption{Results of augmenting semantic recovery with additional $textEnc$ functions and metadata.}
    \label{fig:rq3_results}
\end{figure}

\begin{figure}[!t]
    \centering
    \includegraphics[width=0.45\textwidth]{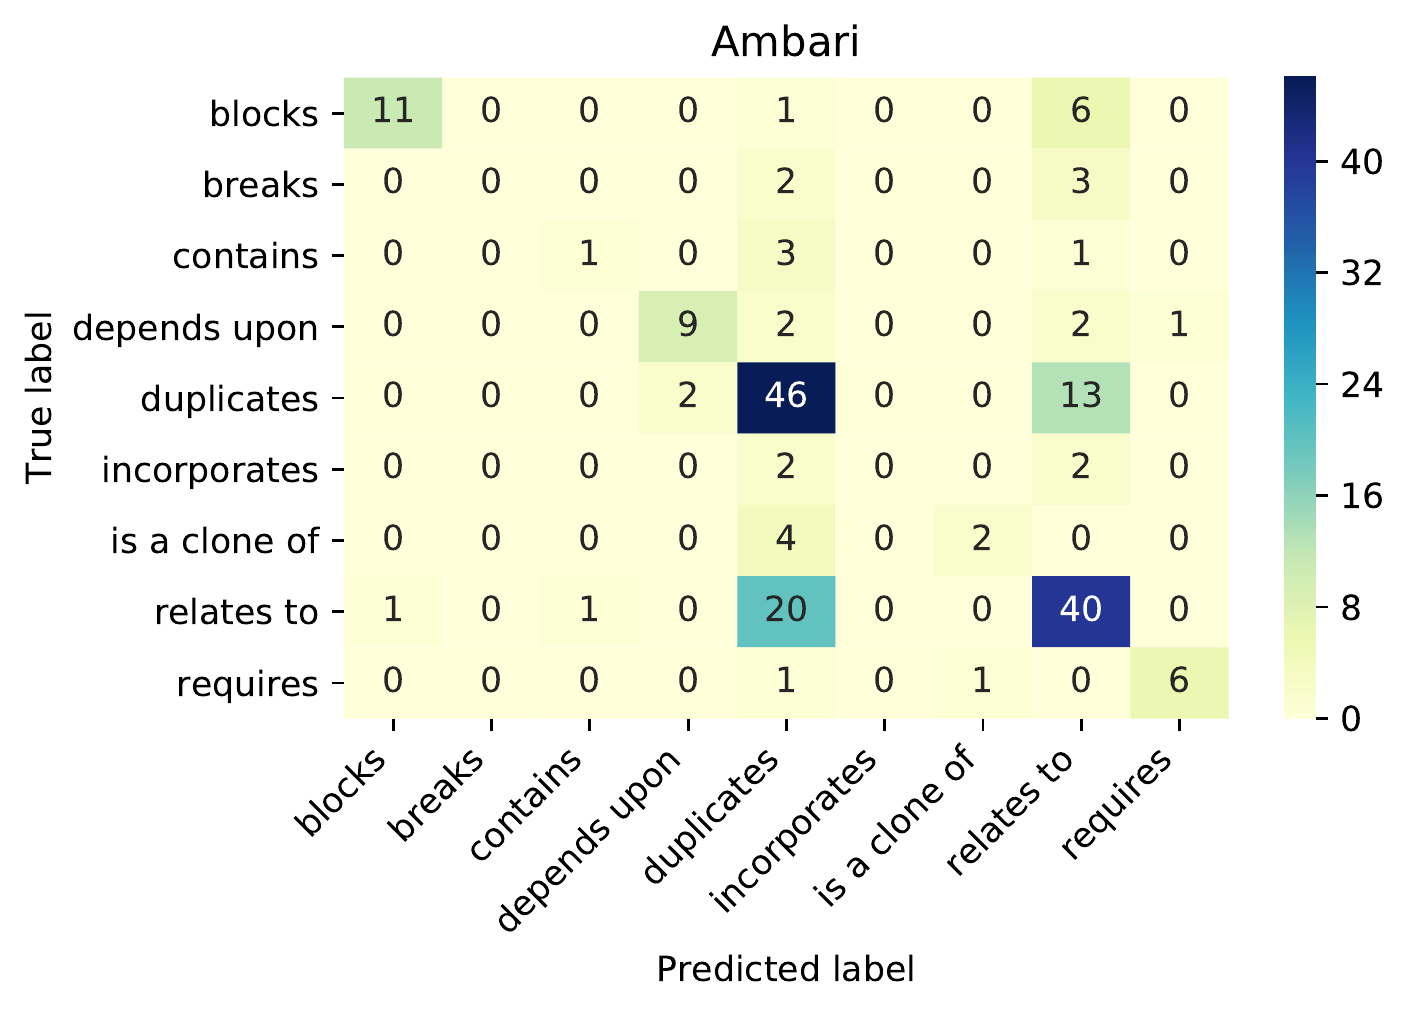}
    \includegraphics[width=0.45\textwidth]{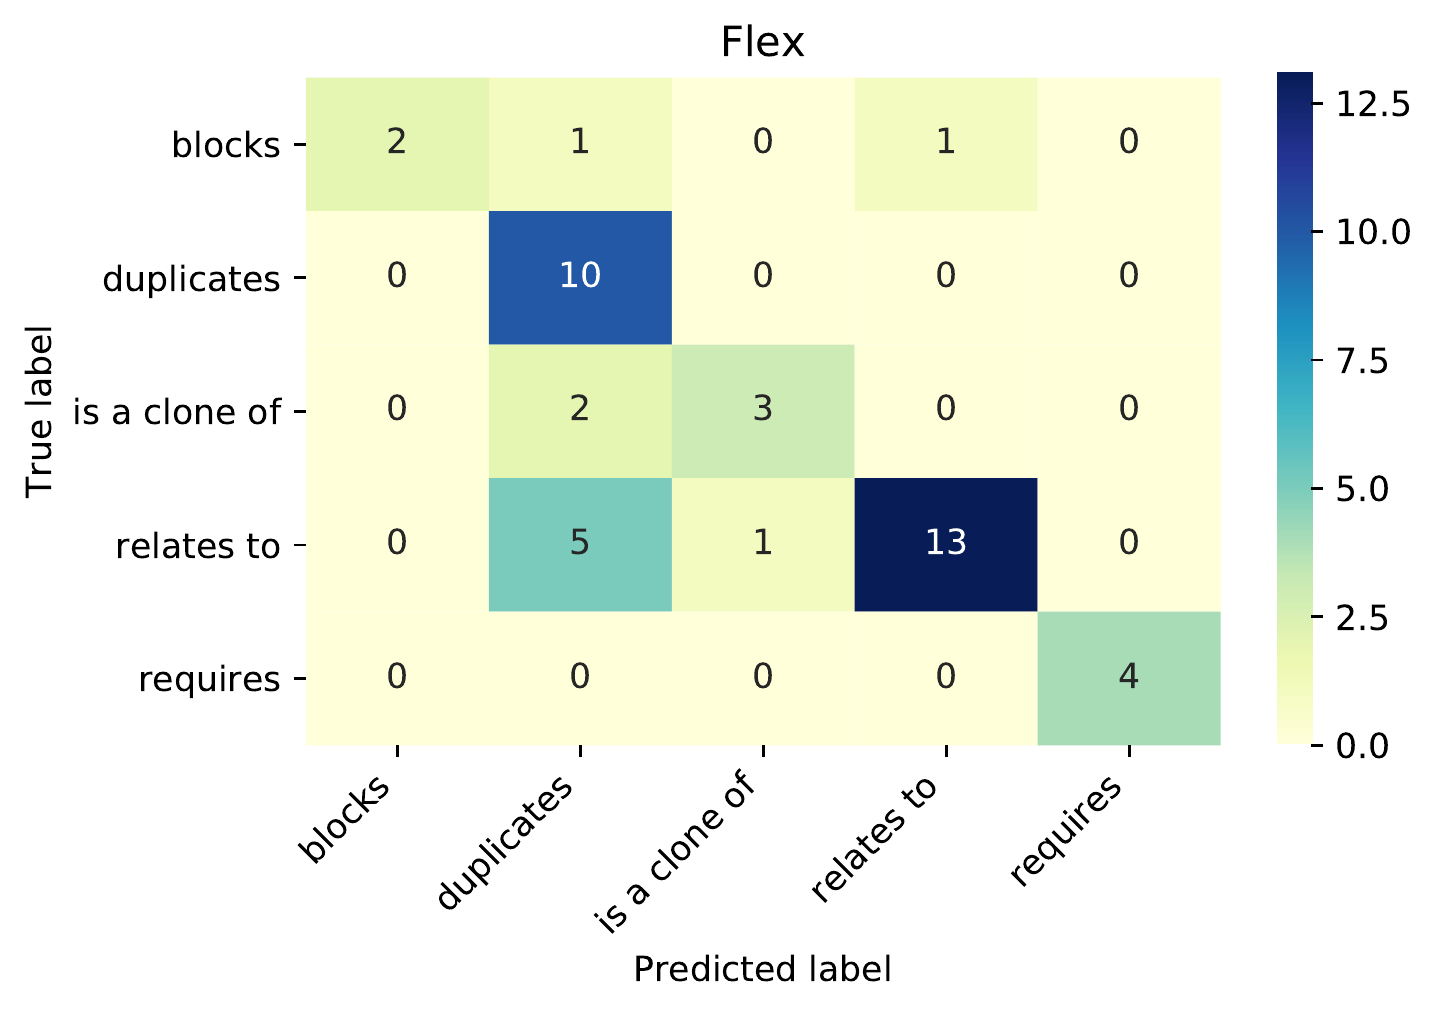}
    \includegraphics[width=0.45\textwidth]{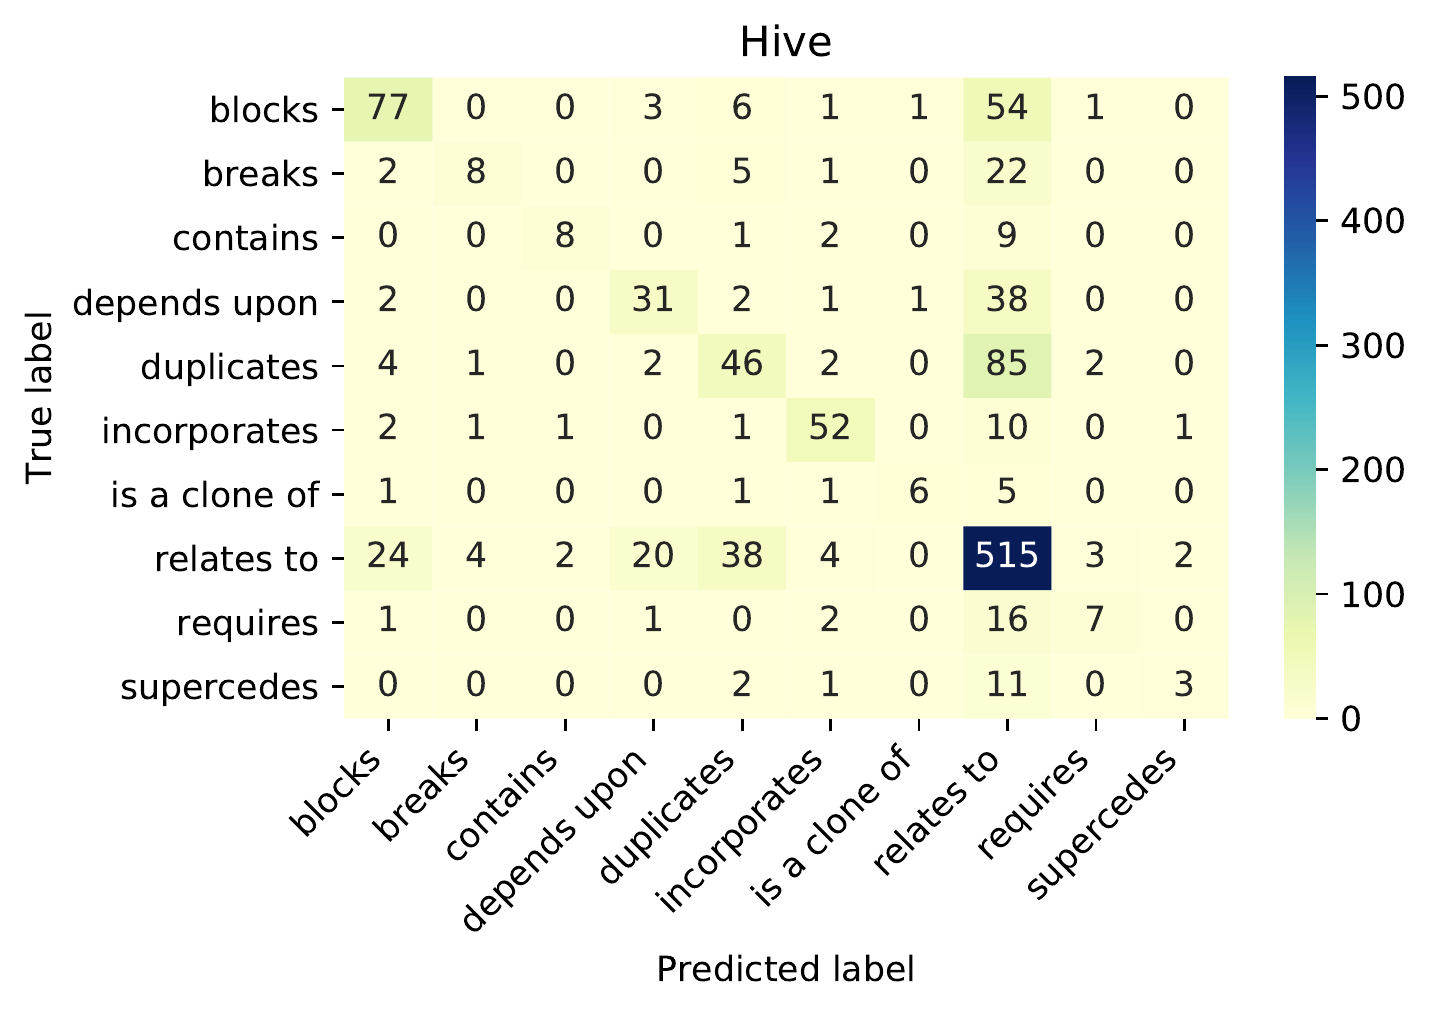}

    \caption{Confusion Matrix of the best performing configurations: \newline Hive (LR using $textEnc_{tfidf}$ + metadata with hyper-parameter tuning), \newline
    Flex (NN using $textEnc_{stack}$ + metadata with hyper-parameter tuning), \newline
    Ambari (RF using $textEnc_{tfidf}$ + metadata with hyper-parameter tuning)}
    \label{fig:confusion_best}
\end{figure}

Figure \ref{fig:rq3_results} shows the results of adding both metadata and additional text encoding functions. Each bar in this figure represents the distribution of achieved weighted F1 score for the input features for one project when using different classifiers and their configurations. The first observation is that word embeddings pre-trained by external text collections all lead to additional variance for the weighted F1 score comparing to using the tf-idf encoding function with the rest of the configuration the same. The benefit of adding features from metadata is more decisive. We have observed notable improvement on both the median and variance of weighted F1 score across all projects. %The variances of applying hyper-parameter tuning across project and classifiers resonate with our findings in Section \ref{sec:recover-semantics}.

The best performing configuration on the Hive dataset is logistic regression with $textEnc_{tfidf}$ and metadata with hyper-parameter tuning, achieving a weighted F1 of $0.630$. On the Flex dataset, the neural network with $textEnc_{stack}$ and metadata tuned with random search performed the best with a weighted F1 score of $0.765$. Finally, on the Ambari dataset, the highest performing combination was the random forest classifier with $textEnc_{tfidf}$ and metadata tuned with the random search, achieving a weighted F1 score of $0.611$. Notably, each dataset had a different optimally performing classifier. The consistent factor is that meta-data combined with hyper-parameter tuning improved performance in each case study project.

Observing the mis-classified samples offers a finer-grained perspective on the task difficulty. Figure \ref{fig:confusion_best} shows the test predictions of the best performing model on each dataset. For both Ambari and Hive, links with various labels can be easily mis-classified as \textit{relates to}. The same case happens for the label \textit{duplicates} for Ambari and Flex. For the \textit{related to} label, it might be caused by the lack of a clear definition of the link semantics when using this label. The links might exhibit heterogeneous features. The label \textit{duplicates} also demonstrate considerable difficulty to reach a satisfying F1 score. In the Flex project for example, although the recall is $100\%$ (all true \textit{duplicates} were recovered), the precision is comparatively low ($10$ of $18$ predicted \textit{duplicates} were actually \textit{duplicates}). This is an interesting finding given that from the textual similarity in our first experiment, \textit{duplicates} seems to be one of two labels for which a high textual similarity is a strong indicator of duplication. The majority ($7$ of $8$) of these , however, were predicted as either \textit{relates to} or \textit{is a clone of} links which might indicate the likely inconsistent use of link labels in the project.

While the performance of the current link semantic recovery solution is far from perfect, as a first step, it might be used to mitigate the effort of assigning link labels from scratch. The prediction can suggest link labels in a way that resembles past usage. Such support can also potentially reduce the inconsistency when manually assigning labels.
